# Supplementary material for: E2FL: Equal and Equitable Federated Learning
Source: arXiv:2205.10454 source file (2022-08-16)
Supplement: Supplementary file 1 [file FFRL_details.tex]

\section{Missing Details of EEFL}
\subsection{When its time to create a new group} \label{sec:qupdate}
Variable $Q$ shows the number of learned groups so far where it is initialized at 1. We create a new group when based on following: 

\paragraphb{Lowest Loss Method:}If we have a global distinugisher $\tau$ which is a threshold that if a client cannot find a model from existing models that produce loss less than this threshold, this client will ask the server to initiate a new supermask for this user.
Value of $\tau$ shows how much we care about performance of tail users and how much we want to share information between different clients. 
There is a trade-off between performance on local data, and shared information for future unseen data. by decreasing the value of $\tau$ we get more groups of users, but the clients inside each group become smaller so, less information is shared between these users.

\paragraphb{OneShot Method }If the task is not one of the existing tasks, then entropy of the outputs cannot be minimized, so if $\max_q \left( \text{softmax}(-\triangledown_{\alpha} H(p(\alpha)))\right)< \frac{1+\epsilon}{q}$ happens  then the client should ask the server to initialize a new task mask for this user and also for future users of this task.

% \begin{equation}
% \max_i \left( \text{softmax}(-\triangledown_{\alpha} H(p(\alpha)))\right)< \frac{1+\epsilon}{q}
% \end{equation}

\paragraphb{Knowledge Transfer to create a new group} ~\citet{wortsman2020supermasks} proposed to use the scores of previous learned supermasks to create a new supermask when it is needed. They called this technique knowledge transfer. We use the same idea, but with rankings, instead of starting from random, if a client needs to create a new group, it can start from the ranking produced by a majority vote between existing group rankings $R_{g,j\in[q]}^t$.

\subsection{Salient features of \XYZ{} through unawareness}

\paragraphb{Communication Cost of \XYZ{}} Please note that for finding the best group ID, there is no need to send all the rankings to the clients. As we mentioned before, each FSL model is a binary mask of '0's and '1's. So a client only receive the binary masks of the learned groups so far to decide which group it belongs to. 

\paragraphb{Computation Cost of \XYZ{}} Using one-shot ID estimation only needs one forward and backward which makes the ID estimation very fast in case of large numbers of existing groups. In IFCA, we need $q$ forward passes to calculate the loss for all the models to decide which one is providing lower loss.

\paragraphb{Knowledge transfer of \XYZ{} when there is a request for creating a new group} we use the knowledge of previous groups to initialize the new group.

\paragraphb{trade-off between using other group knowledge and your own group knowledge} we provide group-based \XYZ{} to provide better performance for each group but also use other group knowledge.
