# Supplementary material for: E2FL: Equal and Equitable Federated Learning
Source: arXiv:2205.10454 source file (2022-08-16)
Supplement: Supplementary file 2 [file relwork.tex]

\section{Related Works}

Algorithmic fairness has been less extensively studied for FL algorithms. 
In FL, the performance of the global model varies across the network due to heterogeneity in the data that each client owns. 
This concern is called \emph{representation disparity}~\cite{hashimoto2018fairness} and results in unfair performance gaps for the participating clients, i.e., a tail user whose data distribution differs from the majority of the clients does not receive similar performance guarantees. 
The major line of work~\cite{li2019fair, zhang2020personalized, mohri2019agnostic, yu2020salvaging, li2020ditto, smith2017federated} defines FL fairness as providing similar accuracy across FL clients.
Specifically, 
Li et al.~\cite{li2019fair} proposed a formal definition for fairness in FL: a model is more fair when its performance distribution across clients is more uniform, i.e., when  std$\{F_k(w)\}_{k \in [K]}$ is small where std$\{.\}$ is the standard deviation and $F_k(.)$ denotes the local objective function of client $k \in [K]$.

Existing techniques for (mainly,  centralized) fair ML can be broadly classified into the three categories of pre-processing, in-processing, and post-processing~\cite{Mehrabi-fairness}.
The literature on FL fairness is still in its infancy, and the existing techniques can be broadly grouped into the following: 

% Yu et al.~\cite{yu2020salvaging}  show that many users do not get benefit by participating in FL: They  compare the accuracy of local model (trained without any collaboration) with that of the global model, and show that for many users, local models have higher performances. They also show that applying differential privacy or robust aggregation rules (e.g., median~\cite{}) makes this problem worse. 
% To address representation disparity and provide fairness to FL clients, following approaches are proposed:

\paragraphb{Sample Re-weighing Approaches:} 
Inspired by fair resource allocation algorithms for  wireless networks, Li et al.~\cite{li2019fair}  design a federated optimization technique called q-FFL. 
This technique aims at improving FL fairness by  minimizing the aggregate reweighed loss, in a way that the devices with higher loss are given higher relative weights. 
Li et al.~\cite{li2020tilted} use a similar  approach to generalize fairness by suppressing or emphasizing the outliers during loss calculation. 
% When we want a model more fair to outlier, we give them higher weight in calculating loss. 
Zhang et al.~\cite{zhang2020personalized}  deign a flexible personalized FL framework that instead of learning a single global model for all clients, the server keeps all the locally trained models for all iterations. For each iteration, each client can download several of the models, and measure how suitable the downloaded models are for its data distribution. Each client will assign weights to each downloaded model by calculating their loss on her test data and the distance from her local model. 
% Models that gives smaller loss and they are close to the local model get more weights. 
Finally the client computes a weighted average of these models to replace her local model. 
% \blue{can u explain why? e.g., "models with higher loss for the client's data are deemed more useful"}, 
% 
% Mohri~\cite{mohri2019agnostic} argue that current FL tries to optimize one global model for a specific distribution by minimizing the loss with respect to uniform distribution of clients. They show that this optimization introduces high risk of a mismatch with target distribution. 
Alternatively, Mohri~\cite{mohri2019agnostic} design \emph{agnostic federated learning} where the model uses a risk-averse objective optimized for any target distribution formed by a mixture of  client distributions. 
% They show that their algorithm provides good-intent fairness for clients participating in FL.  

\paragraphb{Fine-tuning or Transfer Learning:} Yu et al.~\cite{yu2020salvaging}  propose to fine-tune the global model to make it more fair. Specifically, they suggest using Freeze-base adaptation, which freezes the base layers of the target model and  fine-tunes the top layer, as well as  Knowledge Distillation through the global model.

\paragraphb{Multi-Task Learning (MTL):} Fair federated learning can be thought of as a multi-task learning problem where each protected group is learning a different task. Smith et al.~\cite{smith2017federated}  explore personalized FL with a primal-dual MTL framework that trains a separate model for each client (i.e., task) and tries to find task relationships. This approach is only applicable to small numbers of users and only applies to a convex setting which is not a usual assumption in FL. Li et al.~\cite{li2020ditto} view this problem as a two-task learning problem where local optimization is one task and global optimization is the second task. 
They combine global learning and local learning via a globally-regularized MTL framework which works within a  non-convex setting. 
Their approach  learns a personalized local model for each client by using the  distance form the global model as a regularization term.
