# Supplementary material for: E2FL: Equal and Equitable Federated Learning
Source: arXiv:2205.10454 source file (2022-08-16)
Supplement: Supplementary file 3 [file Bounds.tex]

\section{Generalization Bounds} \label{sec:bounds}
~\citet{mansour2020three} bound the maximum difference between true cluster based loss and empirical cluster based loss for their hypothesis. showed that their generalization bound holds for any clustering algorithm. 
\red{use their bound here}

with probability of $1-\delta$ we have:
where $R_{D.m}(H)$ shows Rademacher complexity of class H over the distribution of $D$ with $m$ samples.
$\hat{D}$ and $D$ shows empirical and true distribution. 

\begin{align}
    \max_{h_1, ..., h_k} |\sum_{j=1}^{n} \frac{m_k}{m} \left(\min_{i\in[k]} L_{D_j}(h_i) -  \min_{i\in[k]} L_{\hat{D_j}}(h_i) \right)| \leq 2\sqrt{\frac{n\log{\frac{2k}{\delta}}}{m}} + 
    \max_{C_1, ..., C_k} \sum_{i=1}^k \frac{m_{C_i}}{m} R_{{Di}_i, m_{C_i}} (H)
\end{align}

\begin{align}
    \max_{h_1, ..., h_k} |\sum_{j=1}^{n} \frac{m_k}{m} \left(\min_{i\in[k]} L_{D_j}(h_i) -  \min_{i\in[k]} L_{\hat{D_j}}(h_i) \right)| \leq \sqrt{\frac{4n\log{\frac{2k}{\delta}}}{m}} + \sqrt{\frac{dk}{m}\log{\frac{em}{d}}}
\end{align}

They showed that for good generalization, the average number of samples per user m/n should be larger than logarithm of the number of clusters, and the average number of samples per cluster m/q should be larger than pseudo-dimension of the overall model. surprisingly it does not depend on the minimum number of samples per clients and instead depends on the average statistics.
