# Supplementary material for: E2FL: Equal and Equitable Federated Learning
Source: arXiv:2205.10454 source file (2022-08-16)
Supplement: Supplementary file 4 [file Exp_min_maj.tex]

\section{Minorities vs Majorities}\label{sec:exp2}
In this section, we compare the performances of different FL algorithms for the minority group G1 and the majority group G6 in Figure~\ref{fig:Allloss2} for FairMNISTRotate dataset. Group G1 has only 8 clients among 1000 clients compared to group G6 which has 257 clients.

% \begin{wrapfigure}{r}{0.5\textwidth}
% \centering
% \vspace{-20pt}
\begin{figure*}[hbt!]
\centering
\begin{subfigmatrix}{2}
\centering
  \subfigure[Minority Group (G1)]{
  \includegraphics[width=0.99\columnwidth]{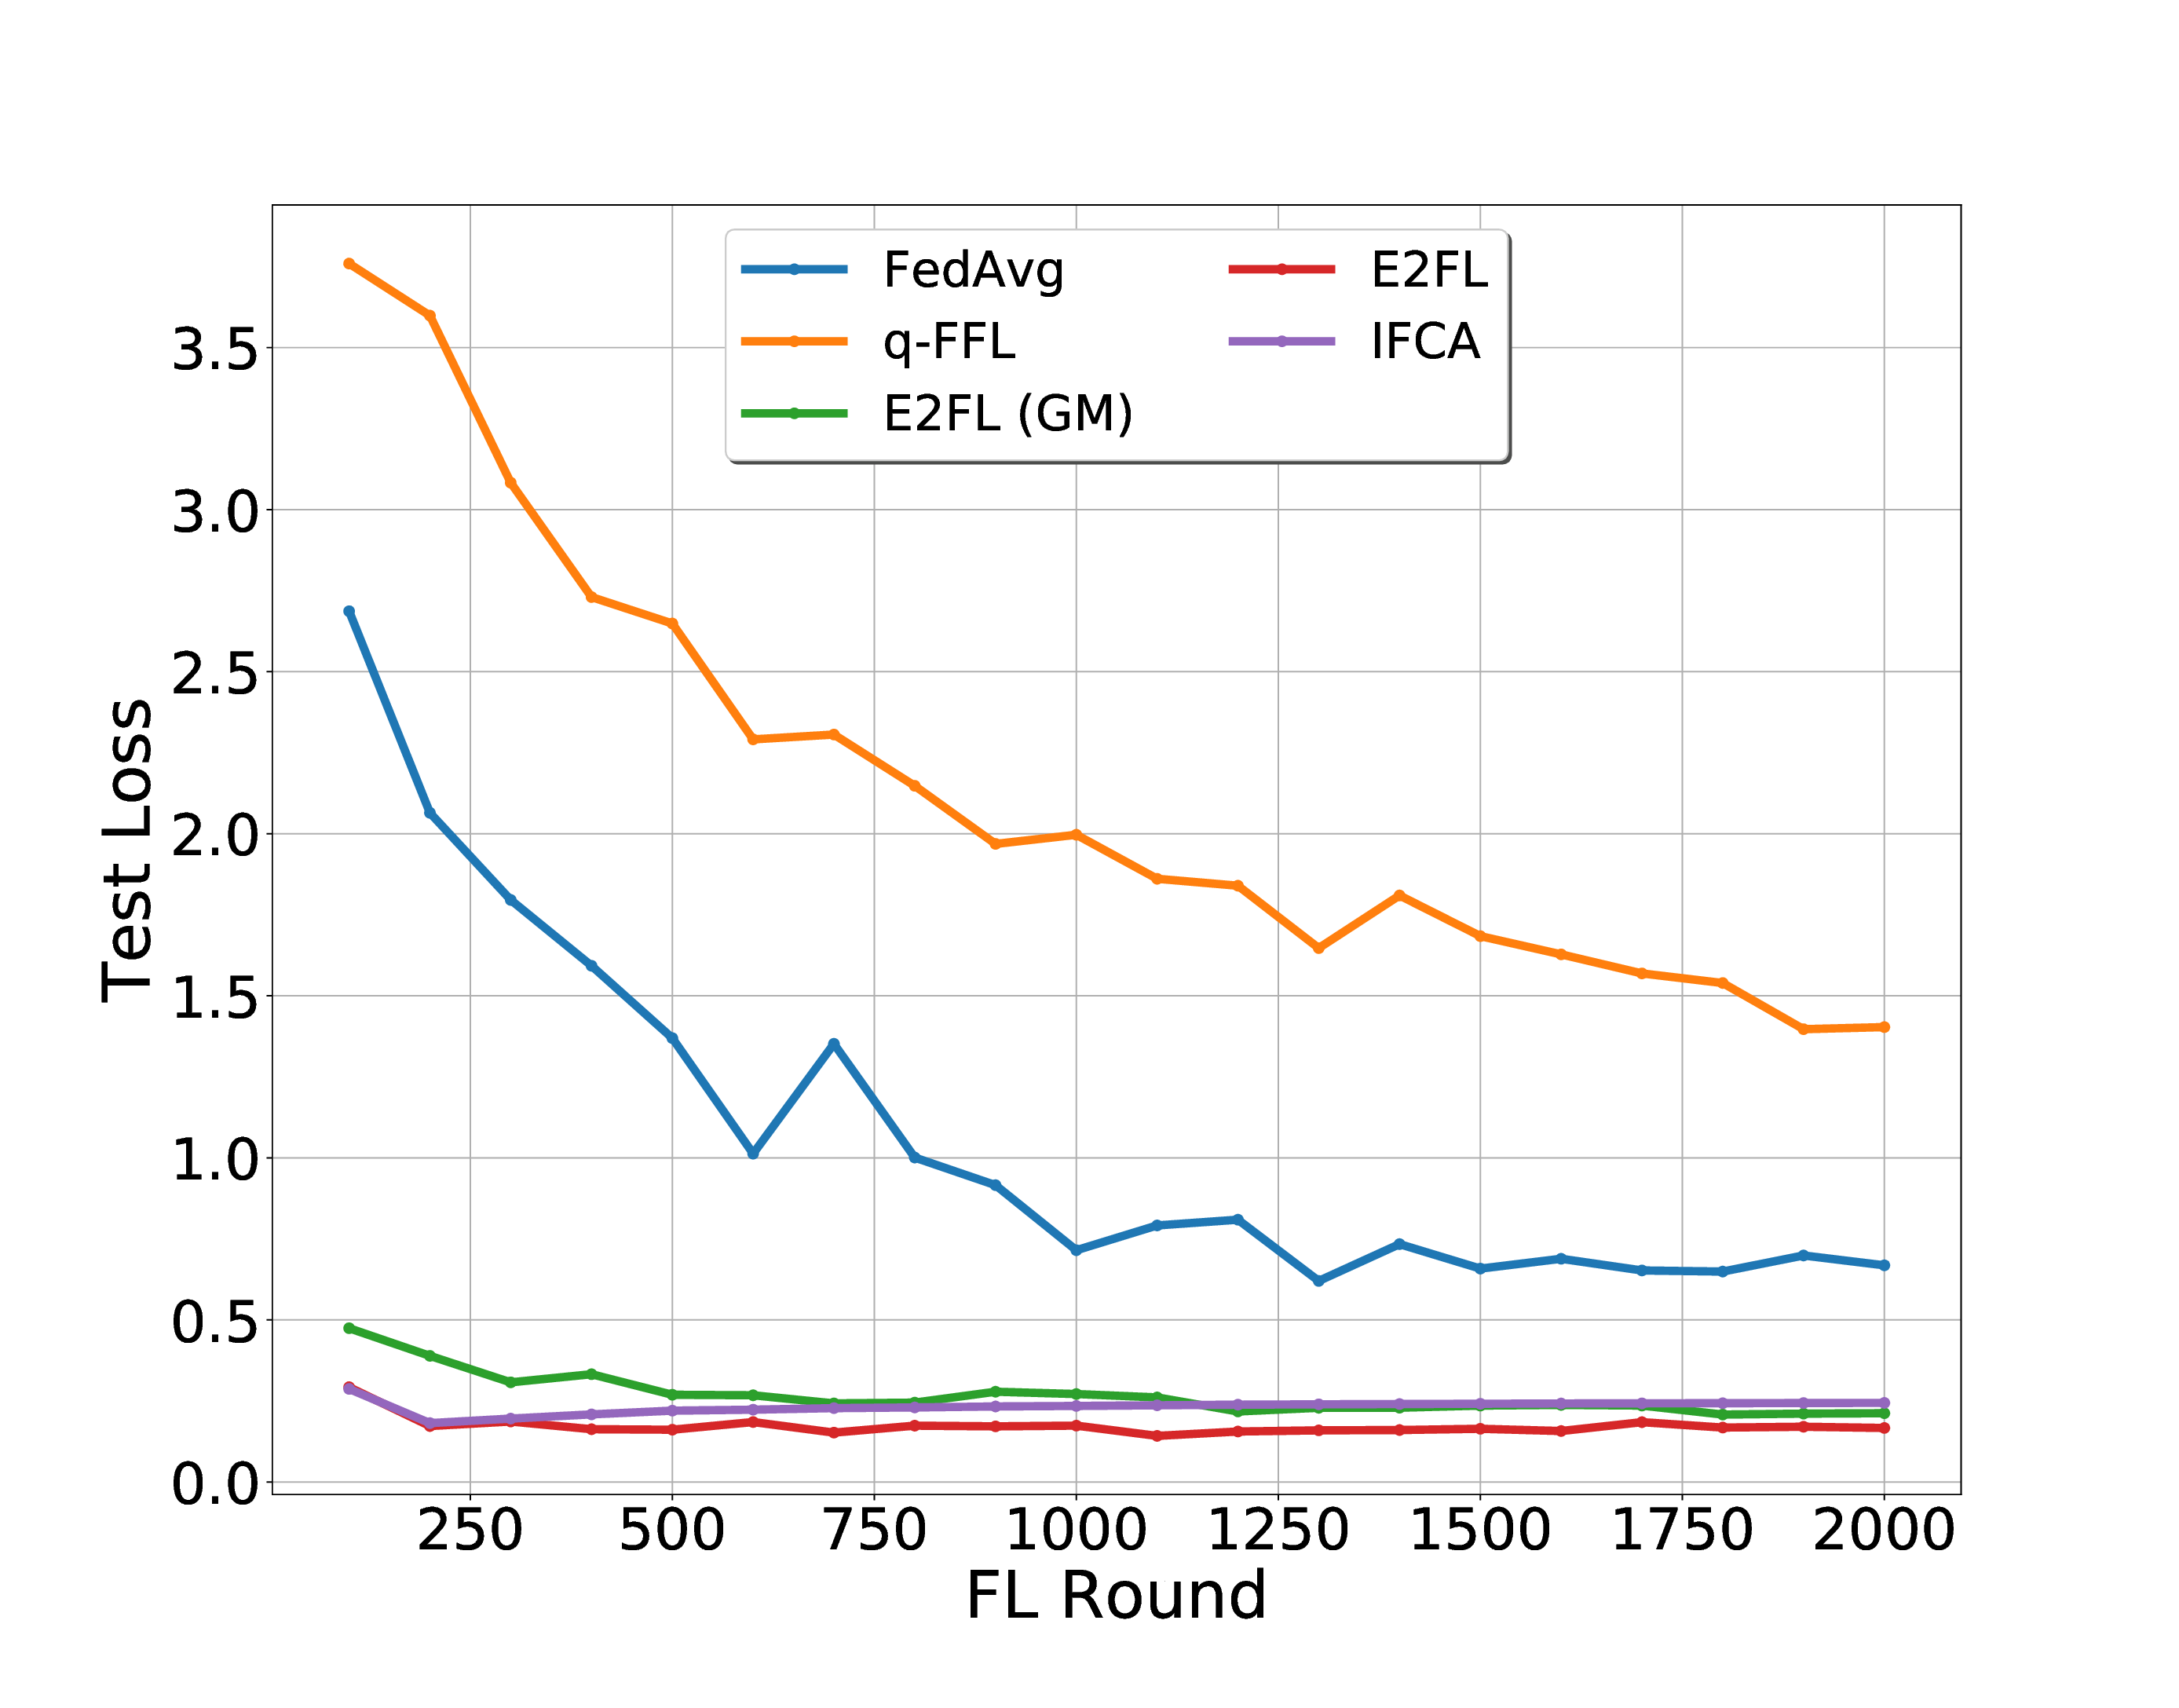}}
  \subfigure[Majority Group (G6)]{
  \includegraphics[width=0.99\columnwidth]{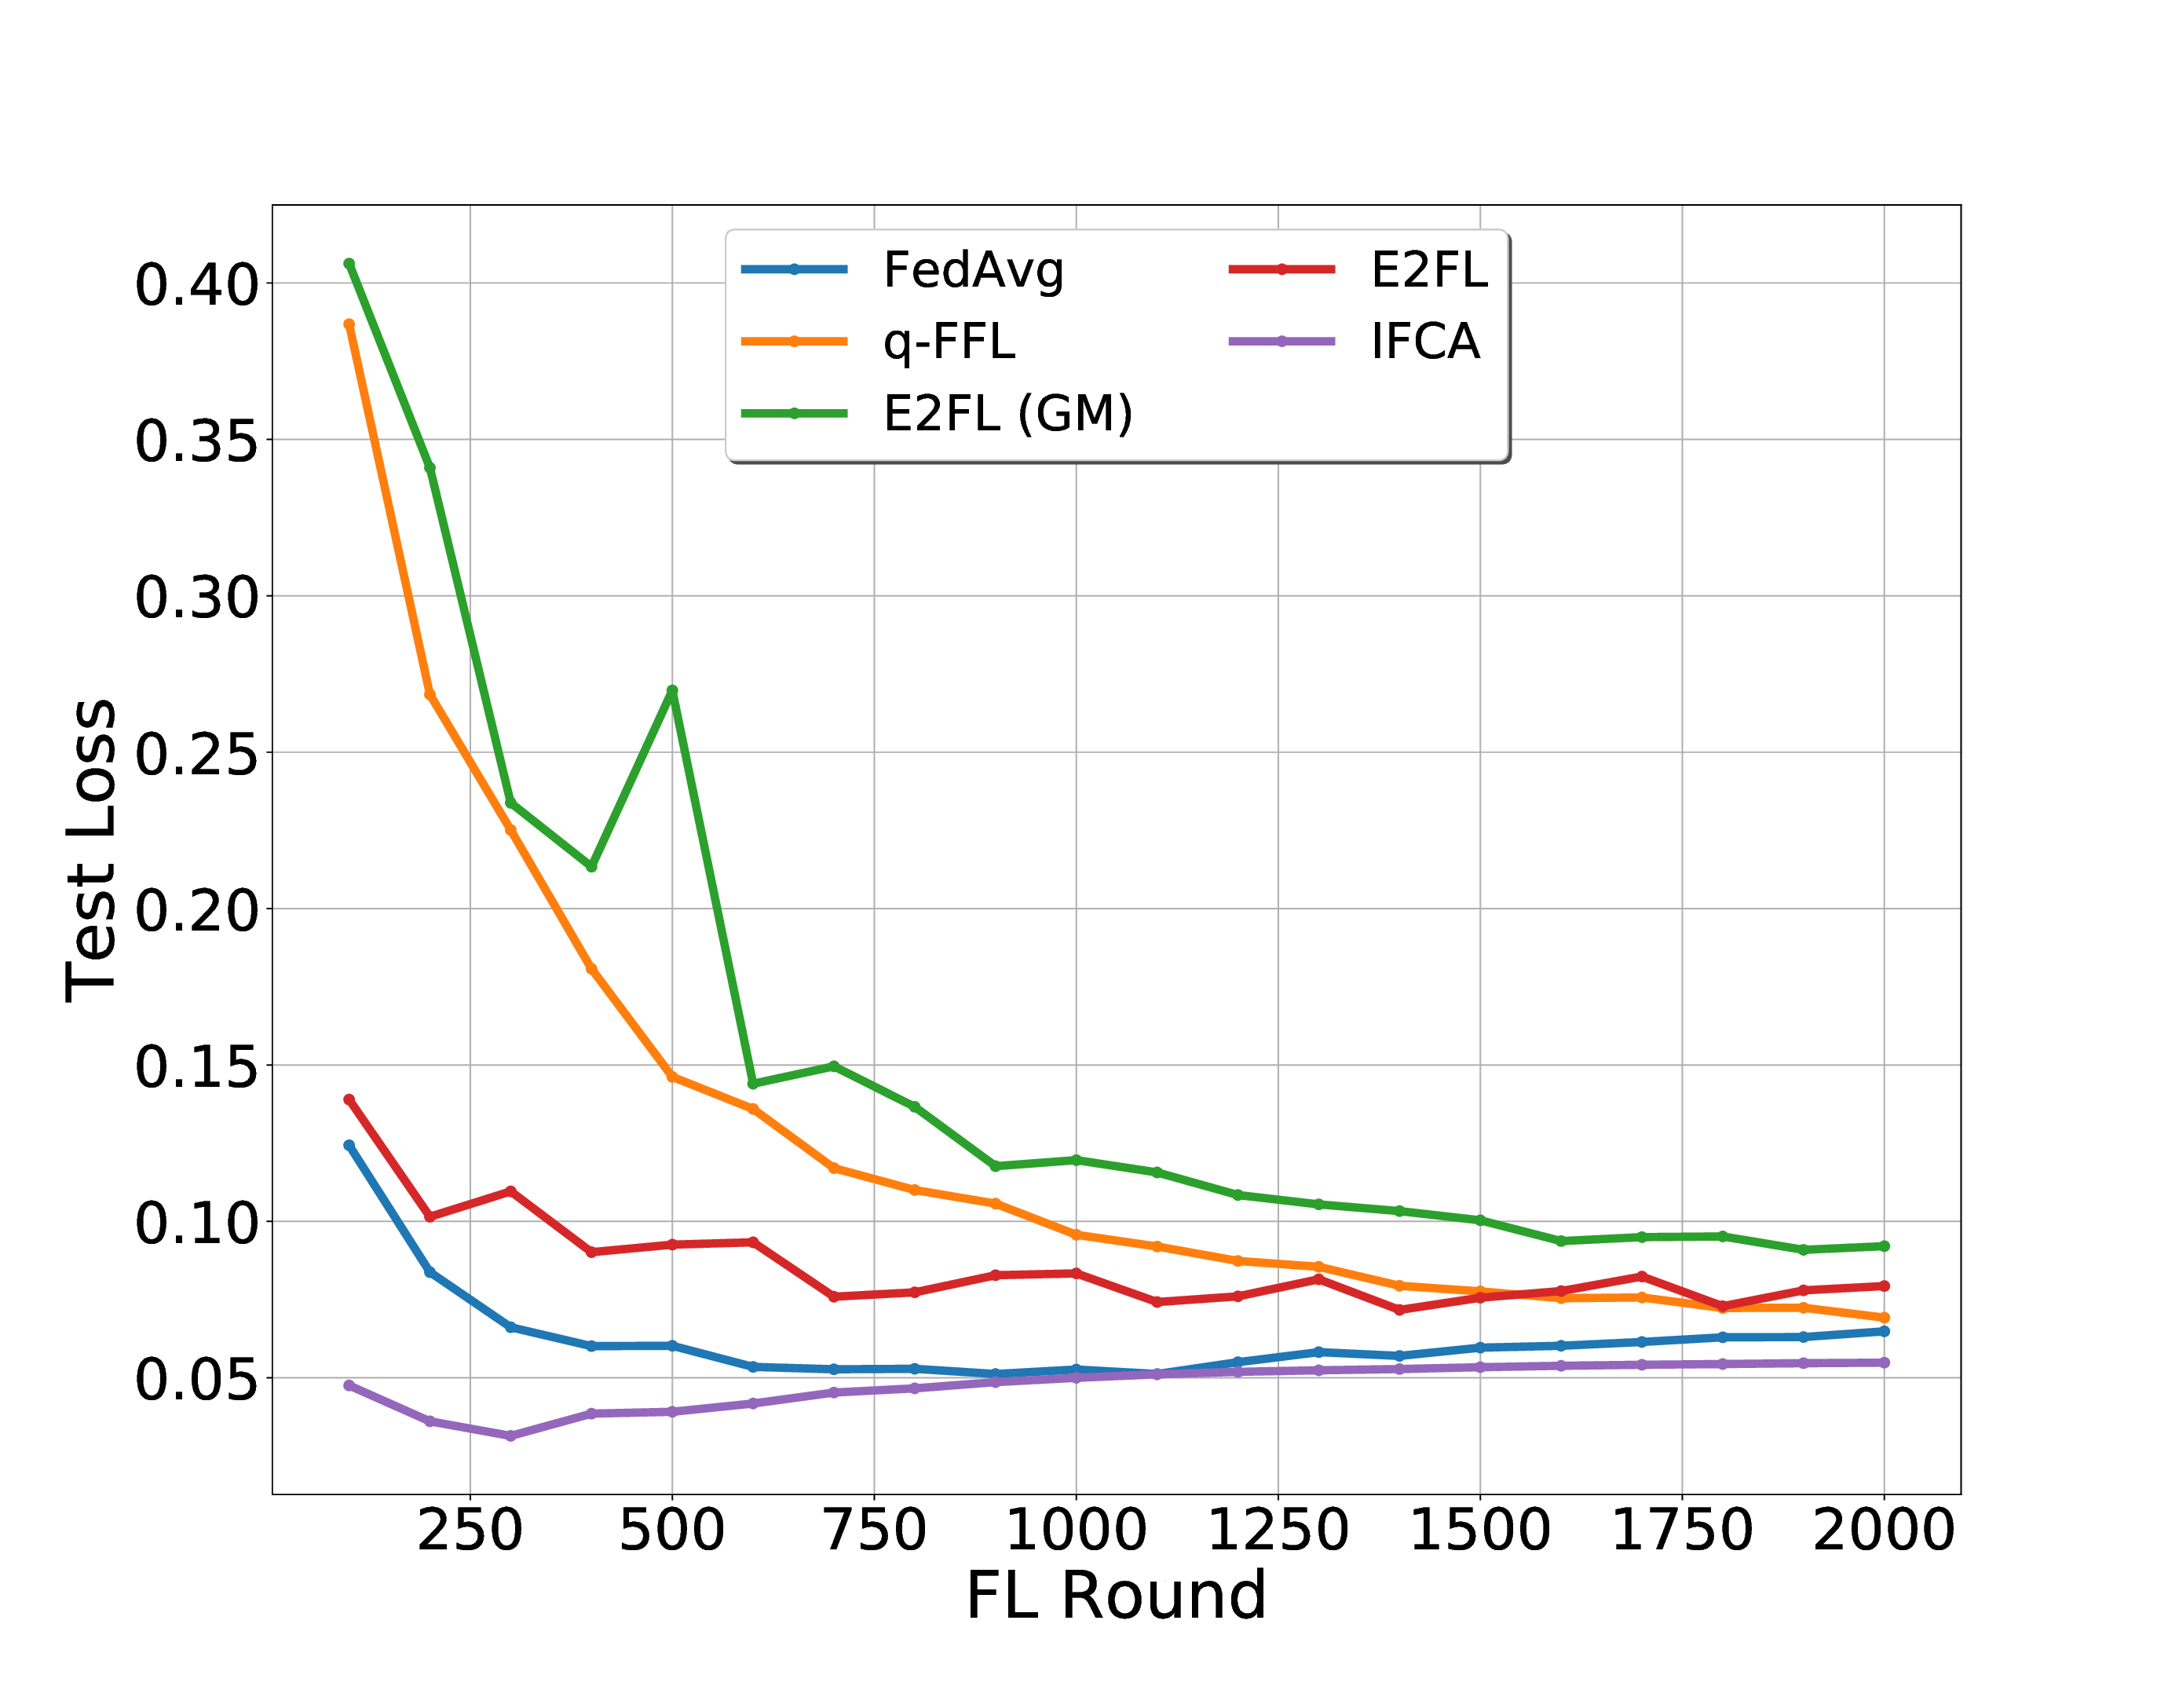}} 
%   \vspace*{-5pt}
%   \subfigure[Majority Group (G6)]{
%   \includegraphics[width=0.40\columnwidth]{Images/G6_Loss_1.eps}} \label{fig:AlllossC}
\end{subfigmatrix} 

% \begin{subfigmatrix}{1}
% \centering
% %   \subfigure[Minority Group (G1)]{
% %   \includegraphics[width=0.40\columnwidth]{Images/G1_Loss_1.eps}} \label{fig:AlllossB}
%   \subfigure[Majority Group (G6)]{
%   \includegraphics[width=0.40\columnwidth]{Images/G6_Loss_1.eps}} \label{fig:AlllossC}
% \end{subfigmatrix} 
\caption{Final test loss for group G1 and G6 for training different FL algorithms on FairMNISTRotate as minority and majority groups}
\label{fig:Allloss2}
\end{figure*}
%     \vspace*{-30pt}
% % \end{figure}
% \end{wrapfigure}
